# Supplementary material for: Your Text Encoder Can Be An Object-Level Watermarking Controller
Source: arXiv:2503.11945 source file (2025-03-15)
Supplement: Supplementary file 1 [file suppl_heatmap_algo.tex]

\begin{algorithm}[!ht]
    \begin{minipage}{\linewidth}
        \caption{Inference: Object-Level Watermarking}\label{alg:object_level_watermarking}
        \begin{algorithmic}[1]
            \Require \textbf{Input} Object to watermark $O^{i}$, Text-to-image prompt $\mathcal{P}$, Diffusion pipeline $\mathcal{D}$, Watermarking token $\mathcal{W}$
            
            \State $\mathcal{D} \gets \mathcal{D} \cup \mathcal{W}$
            \State $\mathbf{x}_T \sim \mathcal{N}(0, I)$
            
            \For{$T = 50, \dots, \tau^*$}
                \State \hspace{1em} $\mathbf{z} \sim \mathcal{N}(0, I)$ if $t > 1$, else $\mathbf{z} = 0$
                \State \hspace{1em} $\mathbf{x}_{t-1} = \frac{1}{\sqrt{\alpha_t}} \left( \mathbf{x}_t - \frac{1 - \alpha_t}{\sqrt{1 - \bar{\alpha}_t}} \epsilon_\theta(\mathbf{x}_t, \mathcal{P}, t) \right) + \sigma_t \mathbf{z}$
            \EndFor
            \vspace{0.5em}

            \For{$t = \tau^*, \dots, 0$}
                \State \hspace{1em} $\mathcal{P} \gets \mathcal{P} + \mathcal{W}$
                \State \hspace{1em} $\mathcal{A}_{O^i}^{(t)} \gets (1 - \lambda) \cdot \mathcal{A}_{O^i}^{(t)} + \lambda \cdot \mathcal{A}_{\mathcal{W}}^{(t)}$
                \State \hspace{1em} $\mathbf{x}_{t-1} = \frac{1}{\sqrt{\alpha_t}} \left( \mathbf{x}_t - \frac{1 - \alpha_t}{\sqrt{1 - \bar{\alpha}_t}} \epsilon_\theta(\mathbf{x}_t, \mathcal{P}, t) \right) + \sigma_t \mathbf{z}$
            \EndFor
            \vspace{0.5em}
            
            \State \Return $\text{watermarked\_image}$
        \end{algorithmic} 
    \end{minipage}
\end{algorithm}

\vspace*{-10pt}
